# Supplementary material for: Classical and Quantum Thermodynamic Systems in Curved Spacetime
Source: arXiv:2005.13965 source file (2020-05-28)
Supplement: Supplementary file 1 [file appendixC.tex]

\chapter{Newton's gravitational constant in d dimensions}
\label{ap:c}

The generalization of Einstein's equations to higher dimensions is automatic, since it is encoded in the tensor indixes. However, Newton's constant has to be generalized as well. In four dimensions, Einstein's equation is
\begin{equation}\label{Ceq1}
G_{\mu\nu} = 8 \pi G T_{\mu\nu}
\end{equation}
where $G_{\mu\nu}$ and $T_{\mu\nu}$ are the Einstein and stress-energy tensors, respectively, and where we have used the units $c=1$. The most simple generalization of (\ref{Ceq1}), and the one we use throughout this work, is
\begin{equation}\label{Ceq2}
G_{\mu\nu} = 8 \pi G_d T_{\mu\nu}
\end{equation}
where the indexes now run from $1,\ldots,d$ instead of $1,\ldots,4$ and $G_d$ is the definition of Newton's constant in $d$ dimensions which leaves Einstein's equation in the form (\ref{Ceq2}). To obtain such definition, we consider the context of Newtonian gravity and recall the Poisson equation for the gravitational field
\begin{equation}
\nabla^2 \phi = k \rho_{m},
\end{equation}
where $\phi$ is the gravitational potential, $k$ is a constant and $\rho_m$ is the density of matter. This equation is the same for $d$ dimensions. Integrating this equation over the space volume $V$ and using the Gauss theorem, we have
\begin{equation}\label{Ceq3}
\int_{V} \nabla^2 \phi \, d^{d-1} x = \oint _{S_{d-2}} (\nabla_{i} \phi) \, n^i \, dS_{d-2} = k \, \int_{V} \rho_m \,d^{d-1}x = k M,
\end{equation}
where $S_{d-2}$ is the boundary surface surrounding the volume $V$, $n^i$ is the unit normal to the surface $S_{d-2}$ and $M$ is the mass contained inside the volume. On the other hand, assuming spherical symmetry, i.e.,
\begin{equation}
(\nabla_{i} \phi) \, n^i  = - g_{r},
\end{equation}
where $g_r$ is the radial component of the gravitational field, one is led to
\begin{equation}\label{Ceq4}
\oint _{S_{d-2}} (\nabla_{i} \phi) \, n^i \, dS_{d-2} = -g_r S_{d-2} \, r^{d-2}.
\end{equation}
Comparing Eq.~(\ref{Ceq3}) and Eq.~(\ref{Ceq4}), yields
\begin{equation}
g_r = - \frac{k}{S_{d-2}} \frac{M}{r^{d-2}}.
\end{equation}
It is clear that $k$ is Newton's gravitational constant in $d$ dimensions apart from some proportionality constant. Simplicity would suggest the choice
\begin{equation}
k = G_d S_{d-2}
\end{equation}
for $k$, as done in \cite{Dvali}, since it gives
\begin{equation}
g_r = - G_d \frac{M}{r^{d-2}}
\end{equation}
which is a straight generalization of Newton's law of gravitation to $d$ spacetime dimensions. However, such choice implies that Einstein's equation must be written as
\begin{equation}
G_{\mu\nu} = \frac{d-2}{d-3} S_{d-2} G_d T_{\mu\nu}
\end{equation}
which is not the desirable form we are interested in. Instead, the choice for $k$ must be the one done in \cite{Myers}, which is
\begin{equation}
k = 8 \pi G_d \frac{d-3}{d-2}
\end{equation}
because, despite leading to the slightly awkward gravitational force law
\begin{equation}
g_r = - \frac{8 \pi G_d}{S_{d-2}} \frac{d-3}{d-2} \frac{M}{r^{d-2}},
\end{equation}
gives the correct form (\ref{Ceq2}) for the Einstein equation. 

This derivation of Newton's constant in a $d$-dimensional spacetime closely follows that of \cite{JV}.
